# Supplementary material for: COVID-BLUeS -- A Prospective Study on the Value of AI in Lung Ultrasound Analysis
Source: arXiv:2509.10556 source file (2025-09-09)
Supplement: Supplementary file 1 [file additional_variables.tex]

\section{Additional clinical variables}

\begin{table*}
\begin{tabular}{lllll}
\toprule
{} &     Total (n=63) & COVID-19 positive (n=33) & COVID-19 negative (n=30) & p-value for group difference \\
                 &                  &                          &                          &                              \\
\midrule \multicolumn{5}{l}{\textbf{Inclusion criteria}} \\ \midrule 
Fever or chills         &        20 (31\%) &                12 (36\%) &                 8 (26\%) &                         0.58 \\
Cough                   &        39 (61\%) &                22 (66\%) &                17 (56\%) &                         0.58 \\
Difficulty breathing    &        59 (93\%) &                31 (93\%) &                28 (93\%) &                         0.68 \\
Loss of taste           &          3 (4\%) &                  3 (9\%) &                  0 (0\%) &                         0.27 \\
Loss of smell           &          3 (4\%) &                  2 (6\%) &                  1 (3\%) &                         0.93 \\
Sore throat             &          2 (3\%) &                  1 (3\%) &                  1 (3\%) &                         0.52 \\
Congestion              &  0.0 ($\pm$ 0.0) &          0.0 ($\pm$ 0.0) &          0.0 ($\pm$ 0.0) &                         1.00 \\
Runny nose              &          3 (4\%) &                  1 (3\%) &                  2 (6\%) &                         0.93 \\
\midrule \multicolumn{5}{l}{\textbf{Symptoms}} \\ \midrule 
Earache                 &  0.0 ($\pm$ 0.0) &          0.0 ($\pm$ 0.0) &          0.0 ($\pm$ 0.0) &                         1.00 \\
Wheezing                &  0.0 ($\pm$ 0.0) &          0.0 ($\pm$ 0.0) &          0.0 ($\pm$ 0.0) &                         1.00 \\
Joint pain              &          1 (1\%) &                  1 (3\%) &                  0 (0\%) &                         0.96 \\
Dyspnea                 &        56 (88\%) &                30 (90\%) &                26 (86\%) &                         0.89 \\
Decreased consciousness &          1 (1\%) &                  0 (0\%) &                  1 (3\%) &                         0.96 \\
Confusion               &          3 (4\%) &                  3 (9\%) &                  0 (0\%) &                         0.27 \\
Abdominal pain          &          3 (4\%) &                  0 (0\%) &                 3 (10\%) &                         0.20 \\
Nausea                  &        11 (17\%) &                 4 (12\%) &                 7 (23\%) &                         0.40 \\
Vomitting               &         8 (12\%) &                 4 (12\%) &                 4 (13\%) &                         0.81 \\
Diarrhea                &         7 (11\%) &                 5 (15\%) &                  2 (6\%) &                         0.50 \\
Skin rash               &  0.0 ($\pm$ 0.0) &          0.0 ($\pm$ 0.0) &          0.0 ($\pm$ 0.0) &                         1.00 \\
Lymphadenopathy         &  0.0 ($\pm$ 0.0) &          0.0 ($\pm$ 0.0) &          0.0 ($\pm$ 0.0) &                         1.00 \\
Ageusia/Dysgeusia       &          4 (6\%) &                 4 (12\%) &                  0 (0\%) &                         0.15 \\
Anosmia/Hyposmia        &          4 (6\%) &                  3 (9\%) &                  1 (3\%) &                         0.68 \\
Emergency case          &        62 (98\%) &                32 (96\%) &               30 (100\%) &                         0.96 \\
\midrule \multicolumn{5}{l}{\textbf{Pulmonary diseases}} \\ \midrule 
DPLD                    &  0.0 ($\pm$ 0.0) &          0.0 ($\pm$ 0.0) &          0.0 ($\pm$ 0.0) &                         1.00 \\
Cystic fibrosis         &  0.0 ($\pm$ 0.0) &          0.0 ($\pm$ 0.0) &          0.0 ($\pm$ 0.0) &                         1.00 \\
Pneumothorax            &  0.0 ($\pm$ 0.0) &          0.0 ($\pm$ 0.0) &          0.0 ($\pm$ 0.0) &                         1.00 \\
Tuberculosis            &  0.0 ($\pm$ 0.0) &          0.0 ($\pm$ 0.0) &          0.0 ($\pm$ 0.0) &                         1.00 \\
Dyspnea                 &          1 (1\%) &                  0 (0\%) &                  1 (3\%) &                         0.96 \\
Other                   &          2 (3\%) &                  0 (0\%) &                  2 (6\%) &                         0.43 \\
\bottomrule
\end{tabular}
\caption{Additional clinical variables that were removed from \autoref{tab:variables_overview} for the sake of simplicity.}
\end{table*}
